# Supplementary material for: Langevin Markov Chain Monte Carlo with stochastic gradients
Source: arXiv:1805.08863 source file (2019-09-17)
Supplement: Supplementary file 1 [file SuppMat.pdf]

# A second-order Langevin method for noisy gradients: Supplementary Material

May 18, 2018

## 1 Extending *NOGIN* to include mass and temperature information

For enhanced sampling schemes such as tempering it is highly desirable to include information about temperature into the distribution. Similarly we may wish to rescale the momentum by a symmetric positive definite mass matrix $\boldsymbol{M}$ to precondition the dynamics to aid exploration in certain directions. Define a new target distribution

$$\pi_\beta(\boldsymbol{\theta}, \boldsymbol{p}) \propto \pi(\boldsymbol{\theta})^\beta \mathrm{N}(\boldsymbol{p} \,|\, \boldsymbol{0}, \boldsymbol{M}/\beta), \tag{1}$$

for inverse temperature parameter $\beta > 0$. Choosing $\beta = 1$ and $\boldsymbol{M} = \boldsymbol{I}$ recovers the *NOGIN* scheme given in the main article. The dynamics to be integrated are

$$\mathrm{d}\boldsymbol{\theta} = \boldsymbol{p}\,\mathrm{d}t, \qquad \mathrm{d}\boldsymbol{p} = \boldsymbol{F}(\boldsymbol{\theta})\,\mathrm{d}t - \boldsymbol{\mu}(\boldsymbol{\theta})\boldsymbol{p}\,\mathrm{d}t + \sqrt{(2/\beta)\boldsymbol{\mu}(\boldsymbol{\theta})\boldsymbol{M}}\,\mathrm{d}\boldsymbol{W}, \tag{2}$$

with $\boldsymbol{\mu}(\boldsymbol{\theta}) = \gamma \boldsymbol{I} + h\boldsymbol{\Sigma}(\boldsymbol{\theta})/2$ as before. The algorithm is given in Algorithm 1.

**Algorithm 1** *NOGIN*: Noisy Gradient Integrator

**Input:** $\boldsymbol{\theta}_0$, $h > 0$, $\gamma > 0$, $T > 0$, $\boldsymbol{M}$, $\beta > 0$

```
Initialize:  p ~ N(0, M/β),  θ ← θ_0,  λ ← sqrt((1 − e^{−γh})/(1 + e^{−γh}))
for t = 1 to T do
    θ ← θ + h M^{−1} p/2
    F̃ ← F̃(θ),  Σ ← Cov(F̃(θ)),  R ~ N(0, M/β)
    p ← p + h F̃/2 + λR
    p ← ((1 − λ^2) I − (h^2/(4β)) M Σ) ((1 + λ^2) I + (h^2/(4β)) M Σ)^{−1} p
    p ← p + h F̃/2 + λR
    θ ← θ + h M^{−1} p/2
    θ_t ← θ
end for
```

$$\boldsymbol{p} \leftarrow \left((1-\lambda^2)\boldsymbol{I} - \tfrac{h^2}{4\beta}\boldsymbol{M}\boldsymbol{\Sigma}\right)\left((1+\lambda^2)\boldsymbol{I} + \tfrac{h^2}{4\beta}\boldsymbol{M}\boldsymbol{\Sigma}\right)^{-1}\boldsymbol{p}$$

## 2 Proof of second-order

We assume that the target distribution $\pi$ is a normalized probability distribution such that $\nabla \log \pi$ is $C^\infty$ with bounded derivatives at all orders, and the gradient noise has bounded moments at all orders for all $\boldsymbol{\theta}$.

In the case of the *NOGIN*scheme we have a single-step update as the composition of maps

$$\Psi_h((\boldsymbol{\theta}, \boldsymbol{p}) \,|\, \widetilde{\boldsymbol{Z}}) = \Phi^{\mathrm{A}}_{h/2} \circ \Phi^{\widetilde{\mathrm{B}}}_{h/2,\widetilde{\boldsymbol{Z}}} \circ \Phi^{\mathrm{O}}_{\tilde{\boldsymbol{\Gamma}}_h,\boldsymbol{0}} \circ \Phi^{\widetilde{\mathrm{B}}}_{h/2,\widetilde{\boldsymbol{Z}}} \circ \Phi^{\mathrm{A}}_{h/2}(\boldsymbol{\theta}, \boldsymbol{p})$$

where $\widetilde{\boldsymbol{Z}}$ represents the injected and gradient noise and where $\tilde{\boldsymbol{\Gamma}}_h$ is chosen as in (13ma) . We can extricate the force updates using (12ma) to rewrite the step as

$$\Psi_h((\boldsymbol{\theta}, \boldsymbol{p}) \,|\, \widetilde{\boldsymbol{Z}}) = \Phi^{\mathrm{A}}_{h/2} \circ \Phi^{\mathrm{B}}_{h/2} \circ \Phi^{\mathrm{O}}_{\tilde{\boldsymbol{\Gamma}}_h,\widetilde{\boldsymbol{Y}}} \circ \Phi^{\mathrm{B}}_{h/2} \circ \Phi^{\mathrm{A}}_{h/2}(\boldsymbol{\theta}, \boldsymbol{p})$$

where $\widetilde{\boldsymbol{Y}}(\boldsymbol{\theta}) = \mathrm{Cov}(\widetilde{\boldsymbol{Z}}(\boldsymbol{\theta}))^{-1}\widetilde{\boldsymbol{Z}}(\boldsymbol{\theta})$ so that $\mathbf{E}[\widetilde{\boldsymbol{Y}}] = \boldsymbol{0}$ and $\mathrm{Cov}[\widetilde{\boldsymbol{Y}}] = \boldsymbol{I}$. Comparing to the exact update for the O piece in (9ma) and taking expectations we obtain

$$\begin{aligned}\mathbf{E}\left[f\left(\Phi^{\mathrm{O}}_{\tilde{\boldsymbol{\Gamma}}_h,\widetilde{\boldsymbol{Y}}}(\boldsymbol{\theta}, \boldsymbol{p})\right)\right] &= \mathbf{E}\left[f\left(\Phi^{\mathrm{O}}_{\boldsymbol{\Gamma}_h,\boldsymbol{R}}(\boldsymbol{\theta}, \boldsymbol{p})\right)\right] + O(h^3) \\ &= \left(e^{h\mathcal{L}_{\mathrm{O}}} f\right)(\boldsymbol{\theta}, \boldsymbol{p}) + h^3(\mathcal{A}f)(\boldsymbol{\theta}, \boldsymbol{p}) + O(h^{7/2})\end{aligned}$$

for operator $\mathcal{A}$ depending upon $\log \pi$ and its derivatives, with $\boldsymbol{\Gamma}_h = \exp(-h\boldsymbol{\mu}(\boldsymbol{\theta}))$ and $\boldsymbol{R} \sim \mathrm{N}(\boldsymbol{0}, \boldsymbol{I})$. Thus the single-step expectation is

$$v_f((\boldsymbol{\theta}, \boldsymbol{p}), h) = \left(e^{h\mathcal{L}_{\mathrm{A}}/2} e^{h\mathcal{L}_{\mathrm{B}}/2} e^{h\mathcal{L}_{\mathrm{O}}} e^{h\mathcal{L}_{\mathrm{B}}/2} e^{h\mathcal{L}_{\mathrm{A}}/2} f\right)(\boldsymbol{\theta}, \boldsymbol{p}) + O(h^3).$$

This can be written as

$$v_f((\boldsymbol{\theta}, \boldsymbol{p}), h) = \left(e^{h(\mathcal{L} + h^2\mathcal{X})} f\right)(\boldsymbol{\theta}, \boldsymbol{p}) + O(h^3) = u_f((\boldsymbol{\theta}, \boldsymbol{p}), h) + O(h^3)$$

through the Jacobi identity, where the operator $\mathcal{X}$ is explicitly given through the Baker-Campbell-Hausdorff (BCH) formula [1].

## 3 Exactness for Gaussian distributions

This can be demonstrated directly using the update maps in (8ma-9ma). Defining

$$\pi_h(\boldsymbol{\theta}, \boldsymbol{p}) = \mathrm{N}(\boldsymbol{\theta} \,|\, \boldsymbol{\eta}, \boldsymbol{\Omega}) \times \mathrm{N}\left(\boldsymbol{p} \,\middle|\, \boldsymbol{0}, \left(\boldsymbol{I} - \frac{h^2}{4}\boldsymbol{\Omega}^{-1}\right)^{-1}\right)$$

we have

$$\begin{aligned}\Phi^{\mathrm{B}}_{h/2} \circ \Phi^{\mathrm{A}}_{h/2}\,(\boldsymbol{\theta}, \boldsymbol{p}) &\sim \pi'_h(\boldsymbol{\theta}, \boldsymbol{p}) \quad \text{if} \quad (\boldsymbol{\theta}, \boldsymbol{p}) \sim \pi_h(\boldsymbol{\theta}, \boldsymbol{p}) \\ \Phi^{\mathrm{A}}_{h/2} \circ \Phi^{\mathrm{B}}_{h/2}\,(\boldsymbol{\theta}, \boldsymbol{p}) &\sim \pi_h(\boldsymbol{\theta}, \boldsymbol{p}) \quad \text{if} \quad (\boldsymbol{\theta}, \boldsymbol{p}) \sim \pi'_h(\boldsymbol{\theta}, \boldsymbol{p})\end{aligned}$$

and

$$\Phi^{\mathrm{O}}_{\widetilde{\boldsymbol{\Gamma}}_h,\widetilde{\boldsymbol{Y}}}(\boldsymbol{\theta},\boldsymbol{p}) \sim \pi'_h(\boldsymbol{\theta},\boldsymbol{p}) \quad \text{if} \quad (\boldsymbol{\theta},\boldsymbol{p}) \sim \pi'_h(\boldsymbol{\theta},\boldsymbol{p})$$

for the distribution

$$\pi'_h(\boldsymbol{\theta},\boldsymbol{p}) := \mathrm{N}\left(\boldsymbol{\theta} \,\middle|\, \boldsymbol{\eta}, \boldsymbol{\Omega}\left(\boldsymbol{I} - \frac{h^2}{4}\boldsymbol{\Omega}^{-1}\right)^{-1}\right) \times \mathrm{N}\left(\boldsymbol{p} \,|\, \boldsymbol{0}, \boldsymbol{I}\right).$$

Thus we have

$$\Phi^{\mathrm{A}}_{h/2} \circ \Phi^{\mathrm{B}}_{h/2} \circ \Phi^{\mathrm{O}}_{h,\widetilde{\boldsymbol{Y}}} \circ \Phi^{\mathrm{B}}_{h/2} \circ \Phi^{\mathrm{A}}_{h/2}(\boldsymbol{\theta},\boldsymbol{p}) \sim \pi_h(\boldsymbol{\theta},\boldsymbol{p}) \quad \text{if} \quad (\boldsymbol{\theta},\boldsymbol{p}) \sim \pi_h(\boldsymbol{\theta},\boldsymbol{p})$$

as required.

# 4 Computing the integrated autocorrelation time

We consider applying the *NOGIN*scheme to a one-dimensional standard normal distribution $\pi(\theta) = \mathrm{N}(\theta \,|\, 0, 1)$ with constant gradient noise variance $\Sigma(\theta) \equiv C^2$, for constant $C^2$. We may write an update of the *NOGIN*scheme as

$$\begin{bmatrix} \theta_{k+1} \\ p_{k+1} \end{bmatrix} = \boldsymbol{A} \begin{bmatrix} \theta_k \\ p_k \end{bmatrix} + \frac{1}{2}(1+\widetilde{\Gamma})hCR_k \begin{bmatrix} h/2 \\ 1 \end{bmatrix},$$

for $R_k \sim N(0,1)$ and

$$\boldsymbol{A} = \frac{1}{8}\begin{bmatrix} 8 - 2h^2(1+\widetilde{\Gamma}) & (4h - h^3)(1+\widetilde{\Gamma}) \\ -4(1+\widetilde{\Gamma})h & 8\widetilde{\Gamma} - 2h^2(1-\widetilde{\Gamma}) \end{bmatrix}.$$

We shall examine the rate of exploration of the state $\boldsymbol{z}_k = [\theta_k, p_k]^{\mathrm{T}}$ in a direction $\boldsymbol{v} = [v_1, v_2]^{\mathrm{T}}$ by looking at the integrated autocorrelation time of $f(\boldsymbol{z}) = \boldsymbol{z} \cdot \boldsymbol{v}$. If we assume that $C$ is large enough so that all the eigenvalues of $\boldsymbol{A}$ are real, then choosing $\boldsymbol{v}$ to be the eigenvector of $\boldsymbol{A}^{\mathrm{T}}$ with largest associated eigenvalue $\lambda$, the autocorrelation function for $f$ is

$$\mathrm{acf}_f(k) := \frac{\mathbf{E}[(\boldsymbol{z}_0 \cdot \boldsymbol{v})(\boldsymbol{z}_k \cdot \boldsymbol{v})]}{\mathbf{E}[(\boldsymbol{z}_0 \cdot \boldsymbol{v})(\boldsymbol{z}_0 \cdot \boldsymbol{v})]} = \frac{\mathbf{E}\left[(\boldsymbol{z}_0 \cdot \boldsymbol{v})(\boldsymbol{z}_0 \cdot (\boldsymbol{A}^{\mathrm{T}})^k \boldsymbol{v})\right]}{\mathbf{E}[(\boldsymbol{z}_0 \cdot \boldsymbol{v})(\boldsymbol{z}_0 \cdot \boldsymbol{v})]} = \lambda^k,$$

where the expectation is over all initial conditions weighted according to the known invariant distribution given. The IAT $\tau_f$, is

$$\tau_f := 1 + 2\sum_{k=1}^{\infty} \mathrm{acf}_f(k) = 1 + \frac{2\lambda}{1-\lambda}.$$

Plugging in the value of $\tilde{\Gamma} = (1 - C^2h^2/2)/(1 + C^2h^2/2)$ with the explicit eigenvalue $\lambda$ we obtain

$$\tau_f = \frac{8 + (C^2-2)h^2 + h\sqrt{h^2(C^4-4) - 16}}{(C^2+2)h^2 - h\sqrt{h^2(C^4-4) - 16}}.$$

For a fixed $h$ and sufficiently large $C$, we have

$$\tau_f \approx \frac{4}{h^2} + C^2 - 1$$

and hence we expect that the autocorrelation time increases like $C^2$, with changing the stepsize $h$ having a negligible impact on $\tau_f$ when $C$ is large.

# References

[1] E. Hairer, C. Lubich, and G. Wanner. *Geometric Numerical Integration: Structure-Preserving Algorithms for Ordinary Differential Equations.* Springer Series in Computational Mathematics. Springer Berlin Heidelberg, 2013.
